# Supplementary material for: Tiled Bit Networks: Sub-Bit Neural Network Compression Through Reuse of Learnable Binary Vectors
Source: arXiv:2407.12075 source file (2024-07-16)
Supplement: Supplementary file 1 [file 36-speed_analysis.tex]

\section{Inference Speed in Standard PyTorch}

We evaluate the efficiency of \glspl{tbn} by assessing their inference speed on several architectures.  To do this, we implement tiled convolutional and fully-connected modules in standard PyTorch. PyTorch offers the \texttt{expand} method on singleton dimensions, which we utilize during model initialization to tile a 1-dimensional tile into a longer vector. The method reuses the single tile in memory at other points within the longer vector. Unfortunately, we are not able to reshape the expanded tensor without allocating new memory because the vectors stride is not compatible with reshaping; at least one dimension spans across two contiguous subspaces. As a result, during inference we need perform the reshape operation, which creates a new tensor the size of the layer in memory, and deallocates it once the layer is complete. The implementation provided in the section results in no benefit in peak memory usage, since a full layer needs to be loaded.  However, it does result in reduced storage size. 

%In this section we test the speed performance of 

%The tiling operation can be implemented as a lookup which maps a weight to a binary value within the tile vector.  Doing so allows us to reuse the tile values within memory with a constant $\mathcal{O}(1)$ computational cost.  To achieve this, we utilize the expand function in PyTorch to move from a single tile vector to a fully tiled vector representing the entire layer.  During inference, we perform a reshape operation to move from a tiled vector to a multidimensional tensor.  The reshaping operation allocates a contiguous memory block for the new tensor, causing a slight performance drop in PyTorch.  The expand method can only operato on singleton dimensions, while individual tiles operate over multiple dimensions.  As a result, we need to 

We perform our experiments on models with full-precision weights, comparing the tiled models to identical models containing standard modules.  We measure the performance in frames per second (FPS), a standard speed measurement technique, over 1000 random samples.

\textbf{Results.}
Table \ref{fps} shows the results of our experiments over five different architectures. We conduct 5 trials for each model and report the mean for each.  The standard deviation is less than 1 for all models. Our results confirm our hypothesis that reshaping and contiguous memory allocation results in a slight drop in performance compared to a dense model of the same structure.  Despite this, the difference is negligible -- less than 2.5\% across all experiments.  We note that further kernel optimizations could be achieved in lower level code to achieve better performance results in \glspl{tbn}.

\begin{table}[h]

\centering

\begin{tabular}{c c c c} 
 \hline
Model & \thead{Num. Tiled\\ Layers}  & \thead{Full-Precision\\ FPS} & \thead{Tiled Model\\ FPS}\\ \hline
 ResNet-18&21 & 302.6&298.9 \\
  ResNet-50&54 & 120.5&117.9\\
 MLPMixer&26&393.61&385.3\\
Swin-t &53&130.2&128.9\\
PointNet& 18 & 392.1&411.5\\
 \hline

 \hline
\end{tabular}
\caption{
\textbf{Speed Analysis}: We compare the \gls{fps} of various architectures when using tiling for linear and convolutional layers and compare it to standard models without tiling. We find that the memory allocation from constructing the layer weights from a tile results in a 0.1\% to 2.4\% decrease in speed, however other kernel optimizations have not been added.}\label{fps}
\end{table}
