# Supplementary material for: Tiled Bit Networks: Sub-Bit Neural Network Compression Through Reuse of Learnable Binary Vectors
Source: arXiv:2407.12075 source file (2024-07-16)
Supplement: Supplementary file 2 [file additional-results.tex]

\section{Additional Results}

We summarize the results of VGG-Small with \glspl{tbn} compared to other sub-bit compression models in Table \ref{cifar10results_additional}. \glspl{tbn} perform competitively with SNN, Spark, and MST, with similar compression rates.

\begin{table}[h]
\scalebox{0.915}{
\centering

\begin{tabular}{c|c c c c } 
%\hline%\hline
 % \multicolumn{5}{c}{\thead{\textbf{CIFAR-10}} }\\    \hline
 \hline
 Model & Method & \thead{Bit-Width\\ (Savings)}  & \thead{\#Params\\ (M-Bit)} & \thead{Test Acc.\\ (\%)}\\
 \hline

 {\multirow{8}{*}{\footnotesize{\thead{VGG\\Small}}}}
 &\footnotesize{Full-Precision} & 32 &  146.24 & 92.7\\
&IR-Net & 1 & 4.656 & 91.3\\
&SNN& 0.440 \footnotesize{\textcolor{blue}{(2.3x)}}&2.032&91.9\\
&Spark*&0.440 \footnotesize{\textcolor{blue}{(2.3x)}}&2.032&90.8\\
&MST*&0.119 \footnotesize{\textcolor{blue}{(8.4x)}}&0.556&91.5\\
\cline{2-5}
&\rowcolor{aliceblue}\gls{tbn}\textsubscript{4}& 0.288 \footnotesize{\textcolor{blue}{(3.5x)}} & 1.340 & 92.6\\
&\rowcolor{aliceblue}\gls{tbn}\textsubscript{8}&0.131 \footnotesize{\textcolor{blue}{(7.7x)}}& 0.722&91.5\\
&\rowcolor{aliceblue}\gls{tbn}\textsubscript{16}&0.117 \footnotesize{\textcolor{blue}{(8.6x)}}&0.520& 90.2\\
 
 \hline
\end{tabular}}
\caption{\textbf{CIFAR-10 Additional Results}: Each result is averaged over three experimental runs.  * indicates model with binary activations. We denote the tiling compression $p$ of each experiment as \gls{tbn}\textsubscript{p}. Savings (in \footnotesize{\textcolor{blue}{blue}}) indicates the compression from a binary-weight model (1-bit per model parameter).  }\label{cifar10results_additional}
\end{table}
