# Supplementary material for: Tiled Bit Networks: Sub-Bit Neural Network Compression Through Reuse of Learnable Binary Vectors
Source: arXiv:2407.12075 source file (2024-07-16)
Supplement: Supplementary file 3 [file discussion_expanded.tex]

\section{Additional Discussion}

\textbf{Limitations} While \glspl{tbn} maximize sub-bit compression for model storage, they only achieve a fraction of potential memory savings as a result of full-precision activation's. Many \gls{bnn} architectures binarize both weights and activation's to maximize computational savings, however we only consider models with full-precision activation's. Full-precision activation's enable better performance across most tasks, and especially in Transformer models (see Section \ref{vision_transformers}). However, we note that \glspl{tbn} still achieve significant memory savings, especially in kernels optimized for the task. Further enhancements could be made to \glspl{tbn} in future work to maximize the memory savings. 

Additionally, \glspl{tbn} only have potential to achieve sub-bit compression for memory and storage; they still require the same number of total operations as a standard binary neural network. Previous sub-bit compression approaches achieve a lower amount of bit-ops, and as a result increase the speed of the models substantially. However, previous work does not work with fully-connected layers. 

\textbf{Applications } \glspl{tbn} are applicable in systems with limited storage space and memory such as IoT devices and embedded systems; the sheer physical size of storage and flash memory can be a burden in devices such as wearables and medical implants. Approaches have been proposed to address memory limitations of such systems \cite{lin2021mcunetv2}, however, no work has looked specifically at reducing storage. \glspl{tbn} maximize storage savings by reducing the number of parameters needed for storing the model to 4x less than the number of model parameters, without a reduction in performance.  Moreover, they achieve memory savings by only requiring the layer tile to be loaded during inference for each layer.
