# Supplementary material for: Tiled Bit Networks: Sub-Bit Neural Network Compression Through Reuse of Learnable Binary Vectors
Source: arXiv:2407.12075 source file (2024-07-16)
Supplement: Supplementary file 4 [file extended_related_work.tex]

\section{Extended Related Work}

\textbf{Binarization}
\glspl{bnn} have a rich history of research.  Subsequent to the work in XNOR-Net \cite{rastegari2016xnor}, XNOR-NET++ fused the activation and scaling factors to learn via backpropagation for enhanced performance \cite{bulat2019xnor}. Dorefa-net focuses on training low bitwidth convolutional neural networks using low bitwidth gradients \cite{zhou2016dorefa}.  ABCNet \cite{lin2017towards} proposed multiple binary bases to improve performance, while Bi-Real use residual connections to reduce information loss \cite{liu2018bi}. Finally, task specific models were proposed such as BiDet for object detection \cite{wang2020bidet}, Qin et al. for keyword spotting \cite{qin2023bifsmnv2}, and Zhao et al. for action recognition \cite{zhao2022pb}.

\textbf{Efficient Machine Learning}
Other work in neural network efficiency includes knowledge distillation \cite{hinton2015distilling, romero2014fitnets}, where a smaller model is trained to replicate the behavior of a larger model,  and neural network pruning, which involves removing various parts of a \gls{dnn}  \cite{he2017channel, frankle2018lottery}. 
Low-rank factorization is a technique in neural networks that approximates weight matrices with reduced-rank forms, offering computational and memory efficiency. Tensor train decomposition introduces specific patterns for hierarchical low-rank approximations \cite{lebedev2014lowrank}. Sparse factorization reduces not only rank but also contributes to smaller memory footprints \cite{howard2017mobilenets}. Dynamic adaptations of rank during training and combining factorization with weight quantization are explored for hardware efficiency \cite{denton2018eigendamage}. %Applications include transfer learning, automated machine learning, and convolutional layers, with implications for robustness and generalization \cite{lebedev2014lowrank,howard2017mobilenets,denton2018eigendamage}.

\textbf{Embedded and On-Device Machine Learning} 
The size and computational requirements of \glspl{dnn} has motivated researchers to improve the compatibility of large models with hardware such as mobile phones and embedded devices (e.g. FGPAs, IoT Sensors)
\cite{cheng2017survey}. Architectural optimizations such as MobileNet \cite{sandler2018mobilenetv2}, ShuffleNet \cite{ma2018shufflenet}, and MCUNet \cite{lin2020mcunet, lin2022device} have been achieved success, including to ease memory constraints via layer patching \cite{lin2021mcunetv2}. 

%knowledge distillation \cite{hinton2015distilling}, pruning \cite{},
