# Supplementary material for: Tiled Bit Networks: Sub-Bit Neural Network Compression Through Reuse of Learnable Binary Vectors
Source: arXiv:2407.12075 source file (2024-07-16)
Supplement: Supplementary file 5 [file full-precisoin-tiling.tex]

\section{Tiled Networks with Full-Precision Weights}

We find that tiling also works with full precision (rather than binarized) weights.  Rather than binarizing the weights with the straight through estimator, we keep the aggregated weights the same. Specifically, we perform two modifications to the training approach to learn full-precision tiled networks: . 
\begin{enumerate}
    \item We average, rather than sum, the reshaped tensor values from parameter $\mathbf{W}$:
     \begin{equation*}
\mathbf{W} = \begin{bmatrix}
\frac{1}{p}\sum_{j=1}^{p} \mathbf{W^{[l]*}_{1j}} \\
\frac{1}{p}\sum_{j=1}^{p} \mathbf{W^{[l]*}_{2j}} \\
\vdots \\
\frac{1}{p}\sum_{j=1}^{p} \mathbf{W^{[l]*}_{qj}}
\end{bmatrix} =
\begin{bmatrix}
s_1 \\
s_2 \\
\vdots \\
s_q
\end{bmatrix} \label{eq2}
 \end{equation*}
 
    \item We do not implement the straight-through estimator on the resulting $\mathbf{W}$ values: $\mathbf{t^{[l]}}=\mathbf{W^{[l]}}=[s_1, s_2,s_i...s_q]$ 
\end{enumerate}

Other parts of the algorithm are not required, such as calculating $\alpha$.  During training, we simply learn a tile from $\mathbf{W}^{[l]}$ scalars; no other parameters are needed outside of $\mathbf{W}^{[l]}$.  

The results of full-precision tiled networks are presented in Table \ref{fp_trans}. We observe a small drop in performance compared to \glspl{tbn}: ViT and Swin-t both perform slightly worse compared to models with binary weights with scalars. Specifically, there is less than a 1\% performance in the tiled models with full precision parameters. We additionally tried adding a learnable scalar to each tile during training, and observed similar results.

We hypothesize that full-precision tiled neural networks could perform better without different algorithmic enhancements.  Moreover, there is potential for \glspl{tbn} and full precision tiled networks in larger scale modeling (e.g. LLMs).  However, we leave this to future work. 

\begin{table}[h]
\centering

\scalebox{1.1}{
\begin{tabular}{c c   c} 
 \hline

 Model & Method  & \thead{Full Precision\\Test Acc.} \\ [0.5ex] 
 \hline
{\multirow{5}{*}{\footnotesize{\thead{ViT}}}}
&\footnotesize{Full-Precision}& 82.5 \\
&\gls{tbn}\textsubscript{4}& 81.5\\
&\gls{tbn}\textsubscript{8}& 80.37\\
&\gls{tbn}\textsubscript{16}& 79.36\\
&\gls{tbn}\textsubscript{32}& 78.0\\

 \hline
{\multirow{3}{*}{\footnotesize{\thead{Swin-t}}}}
& \footnotesize{Full-Precision} & 86.8\\
&\gls{tbn}\textsubscript{4}& 85.5\\
&\gls{tbn}\textsubscript{8}& 84.0\\

\hline

\end{tabular}
}
\caption{\textbf{Full Precision Vision Transformers trained on CIFAR-10}: We assess the performance of a Vision Transformer (patch size 4) and the Swin-t model with tiles that contain full precision weights. Our full precision variation does not use the straight through estimator or $\alpha$ scaling. 
 Instead we only learn a full precision tile. }\label{fp_trans}
\end{table}
