# Supplementary material for: Tiled Bit Networks: Sub-Bit Neural Network Compression Through Reuse of Learnable Binary Vectors
Source: arXiv:2407.12075 source file (2024-07-16)
Supplement: Supplementary file 6 [file gpu_implementation.tex]

\section{GPU Implementation Details}

We implement four total kernels into our models, all for fully-connected layers:
\begin{enumerate}
    \item The standard matrix multiplication kernel provided in the Triton tutorials.  Our only modification is converting the output activation to full-precision (32-bit) tensors. 
    \item A tiled full-precision (32-bit) matrix multiplication kernel.  This kernel assumes we have tiles of 32-bit weights with a compression factor of $p$.  The kernel is fully validated against the Linear module in standard PyTorch. To validate our results, we measure whether the outputs of our tiled kernel and the PyTorch linear module (without bias) are within 0.01 of each other. The kernel implements a matrix multiplication of an $m \times k$ size matrix and a $k \times \frac{n}{p}$ size matrix. We reuse a single tile within the kernel by creating pointers to the $\frac{n}{p}^{th}$ block. 
    
    \item A binary weight kernel.  To implement this, we pack binary values 0 and 1 into \texttt{uint8} data types using the \texttt{numpy} function \texttt{packbits}. The method creates an $\frac{k}{8} \times n$ sized matrix from a $k  \times n$ sized matrix. The kernel performs an interleave operation to repeat the $\frac{k/8}{n}$ dimension  8 times, extracting the $i^{th}$ bit from the \texttt{uint8} corresponding to the values index. This is performed using bit masking. We note that this kernel does not pass validation, and inference yields different results compared to a standard fully connected kernel. However, for research purposes we are able to simulate the memory savings. 
    
    \item A binary weight tiled kernel.  To implement this, we use the logic from the previous two kernels. First, we create a tiled of size $p$, and reshape it into a matrix of size $k \times \frac{n}{p}$ (same as \#2 above). Since standard architectures generally have base 2 sized input features and output features, we are able to achieve this (some layers that don't follow base 2, such as classification layers, are too small to tile). We then pack our $k \times \frac{n}{p}$ sized matrix into a $\frac{k}{8} \times \frac{n}{p}$ sized matrix using \texttt{numpy}. We follow the technical procedures from \#2 and \#3 above. We note that this kernel does not pass validation, and inference yields different results compared to a standard fully connected kernel. However, for research purposes we are able to simulate the memory savings. 
\end{enumerate}

%For our GPU Implementation, we validate the results of our kernel by running our tiled model through an assertion that the PyTorch linear function (with a full-precision weight passed to it) equates to the same result as the result returned by our tiling kernel. Programmatically, we ensure that the models output activation's are similar to each other by comparing their full output tensor. Testing on full precision parameters gives a finer grained analysis 

We include results for the memory savings of \glspl{tbn} in Figure \ref{vit_pointnet} and Table \ref{table:memory_usage} for tiled 32-bit kernel compared to a standard full-precision kernel. Figure \ref{vit_pointnet} shows the memory savings of ViT (trained on CIFAR-10) and PointNet.  The Vision Transformer achieves 2x peak memory savings; the PointNet only achieves very small memory savings. This is the result of the large activation's and inputs into the PointNet model; its parameter sizes are modest compared to the inputs.  The Vision Transformer, on the hand, is able to reduce its large fully-connected layers with tiling, which results in substantial memory improvements. 

Table \ref{table:memory_usage} summarizes the peak memory usage for all models that we tested our full-precision tiled GPU inference kernel on.  The Vision Transformer sized to ImageNet scale data achieved the most substantial improvement: 2.8x reduction in memory as a result of large fully-connected layers.  PointNet and MLPMixer achieved very small memory reductions.
