# Supplementary material for: Tiled Bit Networks: Sub-Bit Neural Network Compression Through Reuse of Learnable Binary Vectors
Source: arXiv:2407.12075 source file (2024-07-16)
Supplement: Supplementary file 7 [file bitops.tex]

\begin{tabular}{|c|c|c|c|}
\hline
\multicolumn{2}{|c|}{Dataset/Model} & Bit-Ops (G) & Test Accuracy (\%) \\
\hline
\multirow{3}{*}{CIFAR10} & ResNet18  & 351.5 & 93.1 \\%cline{2-4}
                         & IR-Net     & 292.9 & 92.9 \\%cline{2-4}
                         & TBN_4        & 219.3 & 93.1 \\
\hline
\multirow{3}{*}{CIFAR10} & ResNet50  & 750.2 & 95.4 \\%cline{2-4}
                         & IR-Net     & 390.6 & 95.1 \\%cline{2-4}
                         & TBN_4        & 415.5 & 94.9 \\
\hline
\multirow{3}{*}{ImageNet} & ResNet34 & 674.8 & 87.3 \\%cline{2-4}
                          & IR-Net     & 112.8 & 70.4 \\%cline{2-4}
                          & TBN_2        & 258.2 & 68.9 \\
\hline
\end{tabular}
