# Supplementary material for: Tiled Bit Networks: Sub-Bit Neural Network Compression Through Reuse of Learnable Binary Vectors
Source: arXiv:2407.12075 source file (2024-07-16)
Supplement: Supplementary file 8 [file code_sample.tex]

\begin{multicols}{1} % Set the number of columns to 1

\begin{lstlisting}[language=Python]
class GetBinaryTiled(autograd.Function):
    @staticmethod
    def forward(ctx, scores, compression_factor):
        score_agg=torch.sum(scores.flatten().reshape((compression_factor,int(scores.numel()/compression_factor))), dim=0)

        out=torch.where(score_agg>0, 1, -1)
        tiled_tensor=out.tile((compression_factor,))
        return tiled_tensor.reshape_as(scores).float()
        
    @staticmethod
    def backward(ctx, g):
        return g , None, None, None
\end{lstlisting}

\end{multicols}
